# Supplementary material for: Experimental electronic phase diagram in a diamond-lattice antiferromagnetic system
Source: arXiv:2412.02213 source file (2024-12-03)
Supplement: Supplementary file 1 [file Supplemental_Materials.pdf]

***Supplemental Materials***

# Experimental electronic phase diagram in a diamond-lattice antiferromagnetic system

Liang-Wen Ji,[1,*] Wu-Zhang Yang,[2] Yi-Ming Lu,[1] Jia-Yi Lu,[1] Jing Li,[1] Yi Liu,[1,3] Zhi Ren,[2] and Guang-Han Cao[1,4,5,†]

[1]*School of Physics, Zhejiang University, Hangzhou 310058, China*
[2]*School of Sciences, Westlake Institute for Advanced Study, Westlake University, Hangzhou 310064, China*
[3]*Department of Applied Physics, Zhejiang University of Technology, Hangzhou 310023, China*
[4]*Interdisciplinary Center for Quantum Information,*
*and State Key Laboratory of Silicon and Advanced Semiconductor Materials, Zhejiang University, Hangzhou 310058, China*
[5]*Collaborative Innovation Centre of Advanced Microstructures, Nanjing University, Nanjing, 210093, China*

## Content

Table S1. Enthalpy and entropy differences between $Co_{8-x}Ni_x[Co_2Ir_{14}]S_{32}$ and $Co_{8-x+y}Ni_{x-y}[Ni_yCo_{2-y}Ir_{14}]S_{32}$

Table S2. Estimation of site inversion degree of Co occupying the *A* site

Figure S1. Temperature dependence of resistivity for $NiIr_2S_4$ and $Co_{1.3-x}Ni_xIr_{1.7}S_4$ ($0.95 \leq x \leq 1.15$)

Figure S2. Temperature dependence of specific heat for $NiIr_2S_4$

Figure S3. Density of states of $Co_{1-x}Ni_x[Co_{0.3}Ir_{1.7}]S_4$ ($x$ = 0.4, 0.6, 0.8, 1)

Figure S4. Band structure of $Co_{1-x}Ni_x[Co_{0.3}Ir_{1.7}]S_4$ ($x$ = 0.4, 0.6, 0.8, 1)

Figure S5. Magnetic susceptibility, isothermal magnetization and specific heat for $Co_{0.3}NiIr_{1.7}S_4$

**Table S1.** Enthalpy and entropy differences between configuration 1 ($Co_{8-x}Ni_x[Co_2Ir_{14}]S_{32}$) and configuration 2 ($Co_{8-x+y}Ni_{x-y}[Ni_yCo_{2-y}Ir_{14}]S_{32}$), with $1 \leq x \leq 8$ and $1 \leq y \leq 2$.

| | $H_1$ (eV/f.u.) | $H_2$ (eV/f.u.) | $\Omega_1$ | $\Omega_2$ | $S_1 - S_2$ ($10^{-5}$ eV/f.u.-K) |
|---|---|---|---|---|---|
| $x = 1, y = 1$ | −42.911 | −42.873 | $C_8^1$ | $C_2^1$ | −1.494 |
| $x = 2, y = 2$ | −42.754 | −42.677 | $C_8^2$ | $C_2^2$ | −3.590 |
| $x = 3, y = 2$ | −42.595 | −42.517 | $C_8^3$ | $C_8^1$ | −2.097 |
| $x = 4, y = 2$ | −42.437 | −42.358 | $C_8^4$ | $C_8^2$ | −0.987 |
| $x = 5, y = 2$ | −42.282 | −42.197 | $C_8^5$ | $C_8^3$ | 0 |
| $x = 6, y = 2$ | −42.126 | −42.035 | $C_8^6$ | $C_8^4$ | 0.987 |
| $x = 7, y = 2$ | −41.970 | −41.879 | $C_8^7$ | $C_8^5$ | 2.097 |
| $x = 8, y = 2$ | −41.815 | −41.725 | $C_8^8$ | $C_8^6$ | 3.590 |

$H_1$ and $H_2$ are obtained from DFT calculations. $S_1$ and $S_2$ are eatimated by $k_B\ln\Omega_1$ and $k_B\ln\Omega_2$, respectively, giving $\Delta S = k_B\ln\Omega_2/\Omega_1$. Thus, the free energy between these two configurations is $\Delta G(T) = G_1(T) - G_2(T) = H_1 - H_2 + k_BT\ln\Omega_2/\Omega_1$. Generally, Ir preferentially occupies the $B$ site, so the disorder between Ni/Co and Ir is not considered in the calculations for simplicity. Note that the formula unit (f.u.) refers to one $AB_2S_4$ unit.

**Table S2.** Estimation of site inversion degree of Co occupying the *A* site in the high-doping region. The deviations of the lattice constant from the linear fit ($\Delta a$) were compared with the differences in ionic radius between Co and Ni ions with and without site inversion, $(R_{Co2+} + R_{Ni3+}) - (R_{Co3+} + R_{Ni2+}) = 0.045$ Å/pair.

| Ni content $x$ | 0.9 | 0.95 | 1.0 |
|---|---|---|---|
| $a$ (Å) | 9.7487(4) | 9.7446(5) | 9.7432(4) |
| $a_{linear}$ (Å) | 9.7319 | 9.7256 | 9.7190 |
| $\Delta a$ (Å) | 0.0168(4) | 0.0190(5) | 0.0242(4) |
| Inversion pairs | 0.373(9) | 0.42(1) | 0.538(9) |
| Inversion degree | 4.6(1) % | 5.3(1) % | 6.7(1) % |

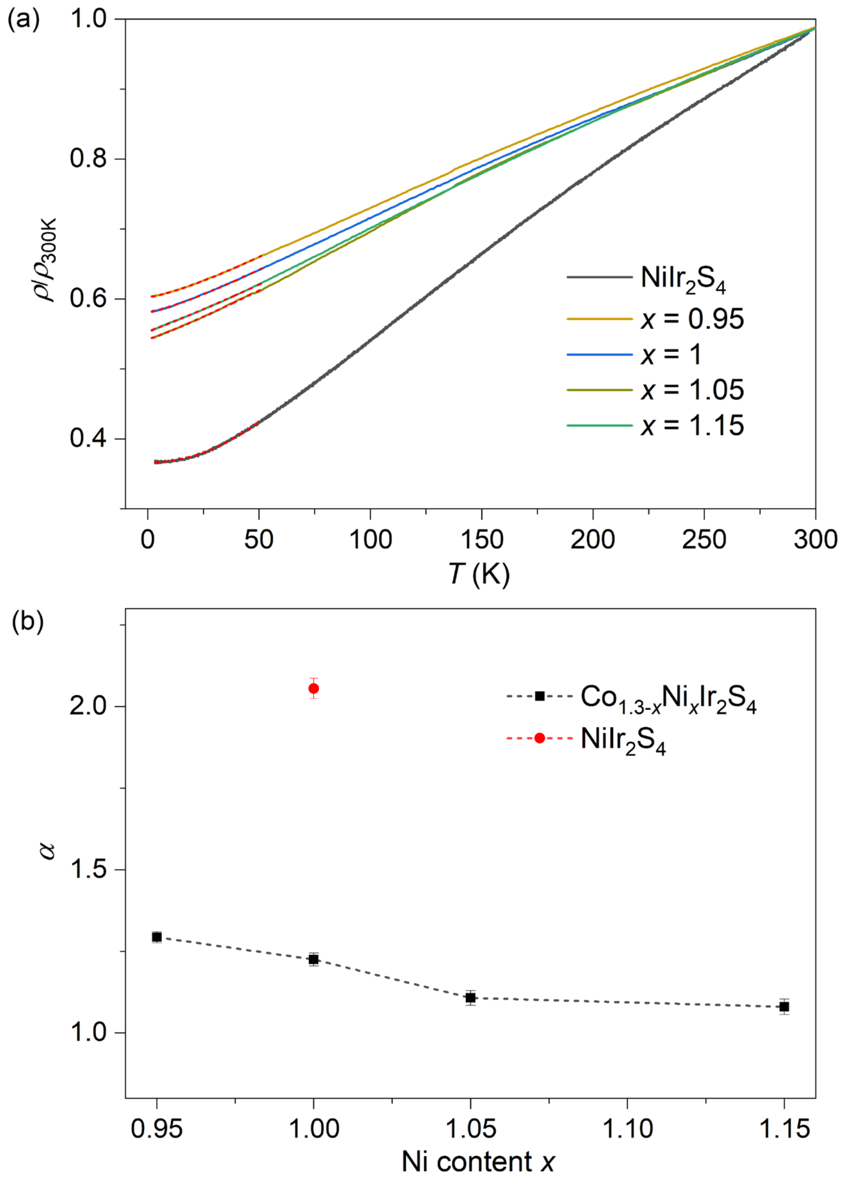


**FIG. S1.** (a) Temperature dependence of normalized resistivity for $NiIr_2S_4$ and $Co_{1.3-x}Ni_xIr_{1.7}S_4$ ($0.95 \le x \le 1.15$). The red dashed lines represent the fit with $\rho = \rho_0 + A'T^{\alpha}$ for data below 50 K. (b) Exponent $\alpha$ for $NiIr_2S_4$ and $Co_{1.3-x}Ni_xIr_{1.7}S_4$.

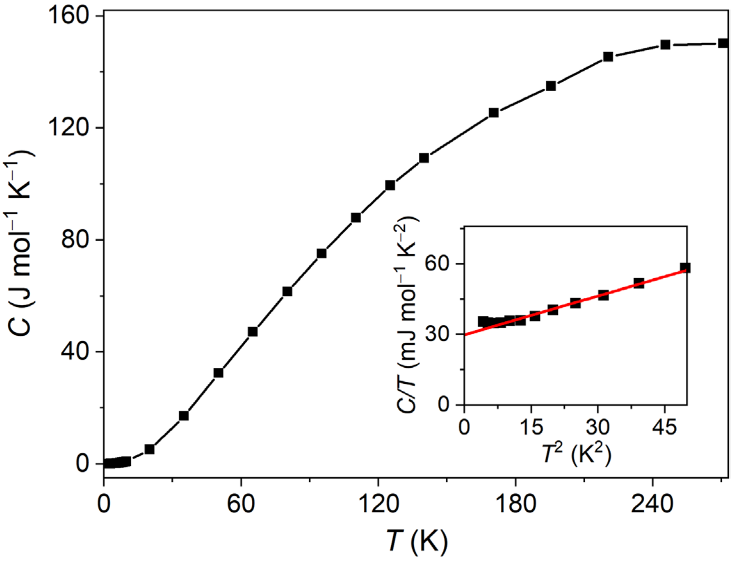


**FIG. S2.** Temperature dependence of specific heat for $NiIr_2S_4$. The inset plots $C/T$ versus $T^2$ in the low-temperature region. The red line represents the fitting with Debye law, which yields $\gamma = 29.05$ mJ mol$^{-1}$ K$^{-2}$ and $\beta = 0.577$ mJ mol$^{-1}$ K$^{-4}$.

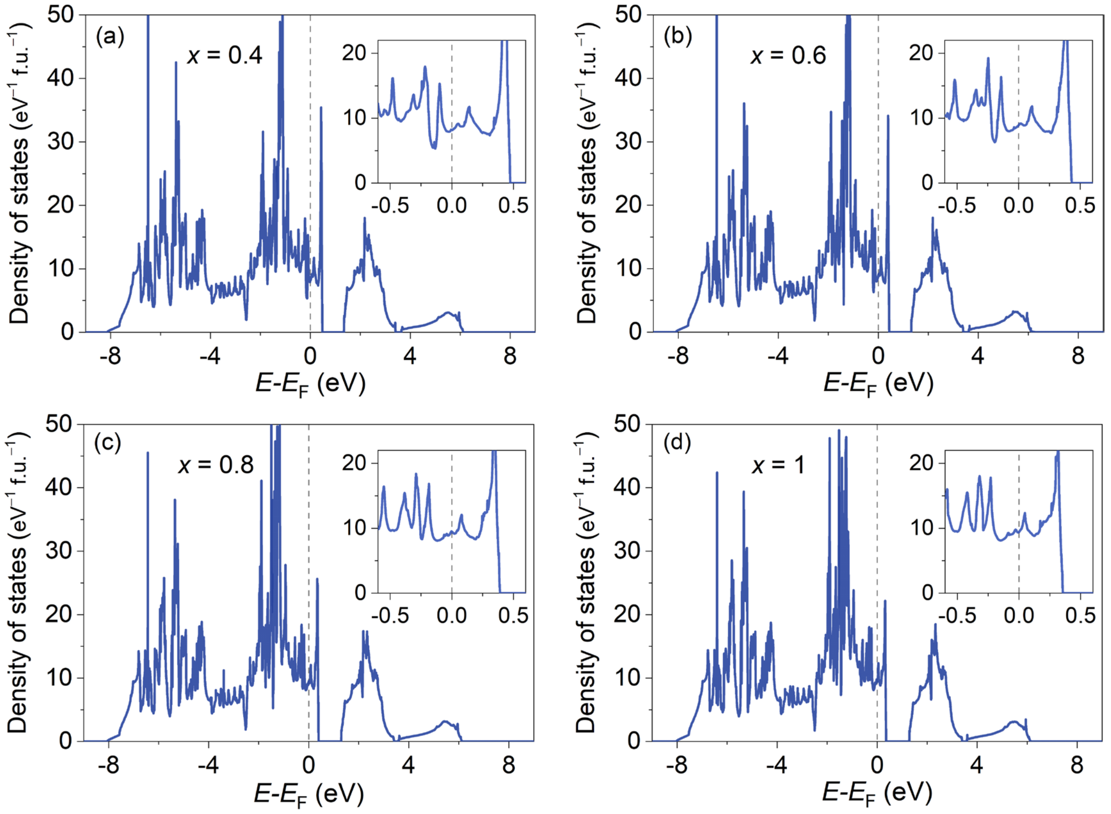


**FIG. S3.** Density of states for $Co_{1-x}Ni_x[Co_{0.3}Ir_{1.7}]S_4$ with $x$ = 0.4, 0.6, 0.8 and 1. The insets show the close-ups around the Fermi energy $E_F$.

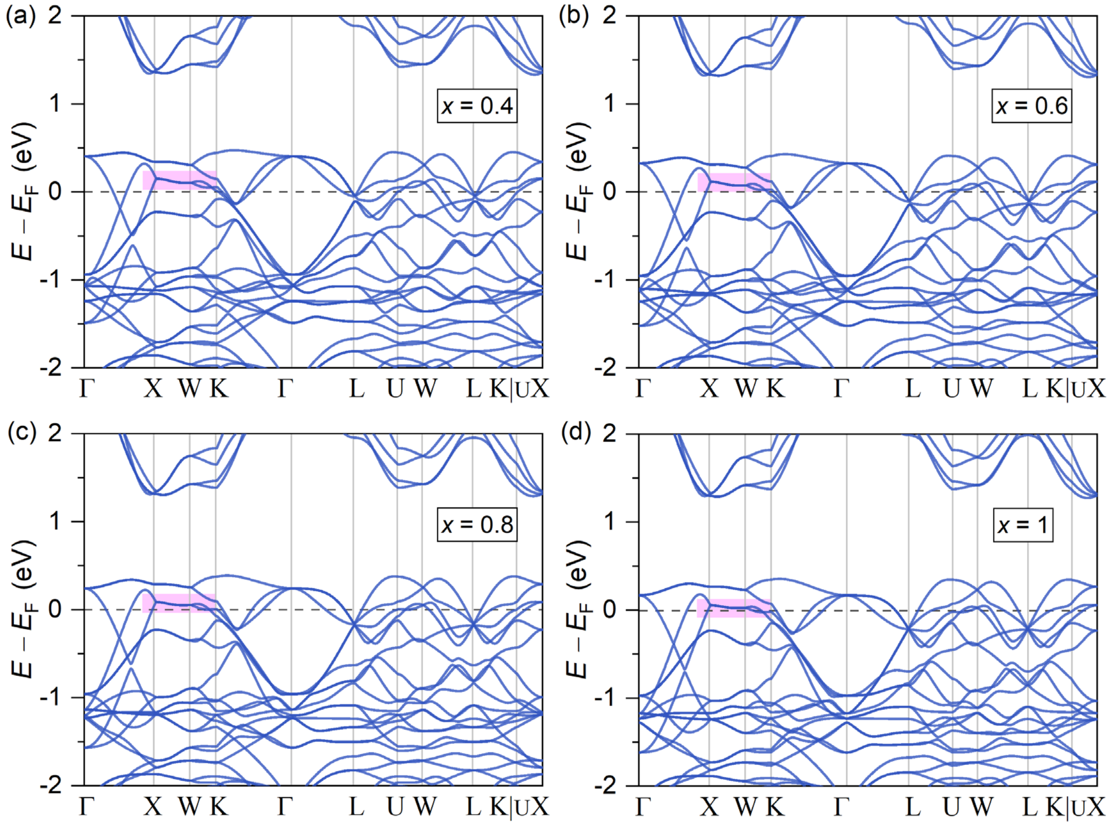


**FIG. S4.** Electronic band structure for $Co_{1-x}Ni_x[Co_{0.3}Ir_{1.7}]S_4$ with $x$ = 0.4, 0.6, 0.8 and 1. The magenta shadows highlight the relatively flat band dispersions near the Fermi energy $E_F$.

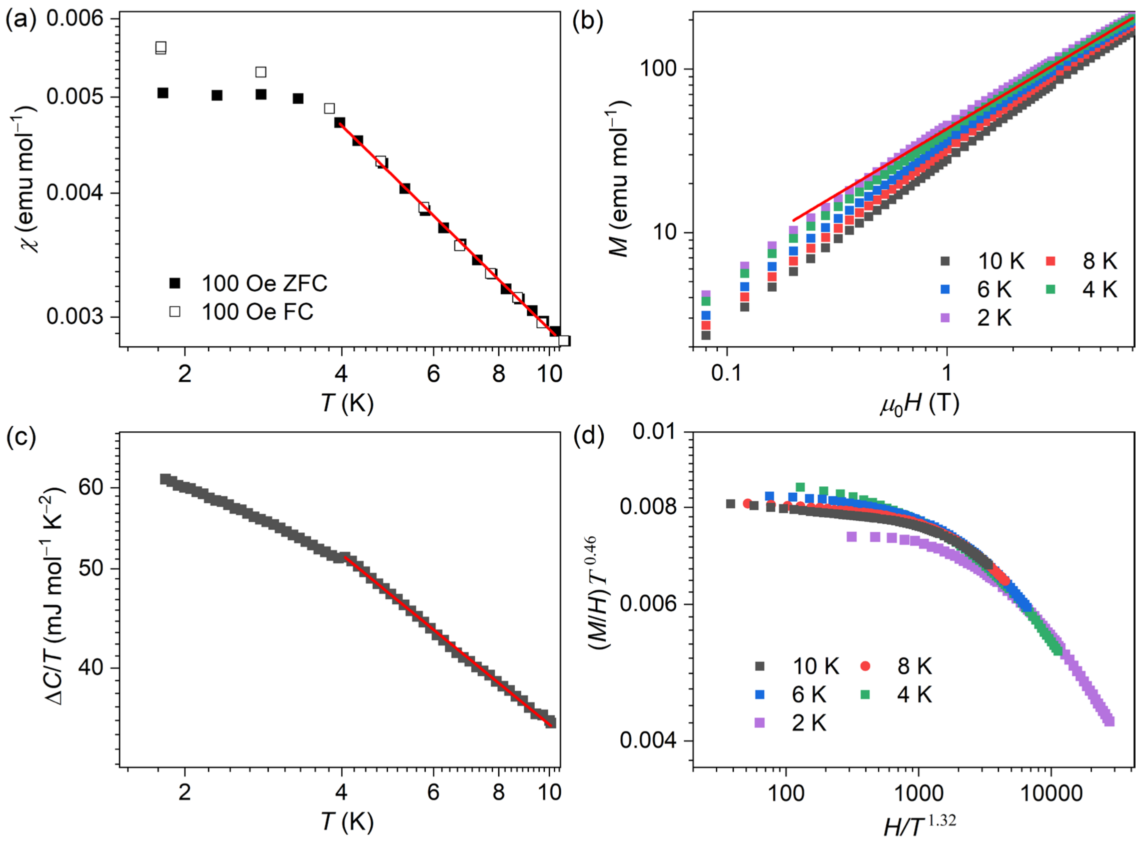


**FIG. S5.** Temperature dependence of magnetic susceptibility (a), isothermal magnetization versus magnetic fields (b), temperature dependence of specific heat (c) for $Co_{0.3}NiIr_{1.7}S_4$. The red line represents a fit with the power law. Here, $\Delta C = (C - C_{\mathrm{lattice}})$ and the lattice contribution of the form $\beta T^3$ has been subtracted from $C(T)$. (d) Scaling of $(M/H)T^{\eta}$ vs $H/T^{\delta}$.
